# Supplementary material for: Decentralized Directed Collaboration for Personalized Federated Learning
Source: arXiv:2405.17876 source file (2024-05-28)
Supplement: Supplementary file 1 [file 09_appendix_odl.tex]

\clearpage
\begin{center}
 \rule{5.6in}{0.7pt}\\ % 4.0
%\vspace{0.2cm}
 {\Large\bf Supplementary Material for \\`` ''}
 \rule{5.6in}{0.7pt}
\end{center}
\appendix

In this part, we provide the supplementary materials including more introduction to the related works, experimental details and results, and the proof of the main theorem.

\begin{itemize}
    \item \textbf{Appendix} \ref{ap:related_works}: More details in the related works.
    \item \textbf{Appendix} \ref{ap:baseline}: More details in the experiments.
    \item \textbf{Appendix} \ref{ap:proof}: Proof of the theoretical analysis.
\end{itemize}
\section{More Details in the Related Works}\label{ap:related_works}
\section{More details in the experiments}\label{ap:baseline}
\section{Proof of Theoretical Analysis}\label{ap:proof}

\subsection{Preliminary Lemmas}

\begin{lemma}[Lemma 23, \cite{pillutla2022federated}]
\label{le:v} 
    Consider $F$ which is $L$-smooth and fix a $v^0 \in \mathbb{R}^d$. 
	Define the sequence $(v^{k})$ of iterates produced by stochastic gradient descent with a fixed learning rate $\eta_v \leq 1/(2K_vL_v)$
	starting from $v^{0}$, we have the bound
	\[
		\E \| v^{K_v-1} - v^{0} \|^2 \le 16 \eta_v^2 K_v^2 \E \|\nabla  F(v^{0})\|^2 + 8 \eta_v^2 K_v^2 \sigma_v^2 \,.
        \]
\end{lemma}

\begin{lemma}[mixing connectivity]\label{th:lemma2}
Suppose that Assumption \ref{assmp:mixing connectivity} holds. Let $\lambda = 1 - n D^{-(K_{u} + 1) \Delta B}$ and let $q = \lambda^{1/((K_{u}+ 1) \Delta B + 1)}$. Then there exists a constant
\[
C < \frac{2 \sqrt{d} D^{(K_{u} + 1) \Delta B}}{\lambda^{\frac{(K_{u} + 1) \Delta B + 2}{(K_{u} + 1) \Delta B + 1}}},
\]
where $ d $ is the dimension of $ \bar{u}^{t}$, $z_i^{t}$, and $ u_i^{0} $, such that, for all $ i=1,2,\dots,m$ (non-virtual nodes) and $ t\geq0 $, 

$$ \|{ {\bar{u}^t} - z_i^{t} } \| \leq C q^t \|{ u_i^{0}}\|  + \eta_u C \sum^t_{s=0} q^{t-s} \|{ \nabla_u F_{i}(z_i^s,v^{s+1})\|}. $$
\end{lemma}

This particular lemma follows after a small adaptation to Theorem~1 in \cite{assran2020asynchronous} and its proof is based on \cite{Wolfowitz1963products}. Similar bounds appear in a variety of other papers, including \cite{nedic2016stochastic,assran2019stochastic}.

\begin{lemma}[Bound of stochastic gradient]
\label{th:lemma3}
We have the following inequality under Assumptions \ref{assmp:smoothness} and Assumptions \ref{assmp:grad-diversity.}:
$$\E \| \nabla_u F_i(z^t_i,v^{t+1}) \|^2 \leq 3 L^2 \E \|z^{t}_i - \bar{u}^t \|^2 +3\delta_u^2 + 3\E\|\nabla_u F(\bar{u}^t,v^{t+1})\|^2 $$
\end{lemma}
\begin{proof}
\begin{eqnarray*}
	\E \|\nabla_u F_i(z^t_i,v^{t+1}) \|^2 & \leq & 3 \E \| \nabla_u F_i(z^t_i,v^{t+1}) - \nabla_u F_i(\bar{u}^t,v^{t+1}) \|^2 +  3 \E \|{ \nabla_u F(\bar{u}^t,v^{t+1}})\| ^2  \\
    &+& 3 \E \|{ \nabla_u F_i(\bar{u}^t,v^{t+1}) - \nabla_u F(\bar{u}^t,v^{t+1}) }\|^2  \notag \\
    &  \overset{\text{Smoothness}}{\leq} & 3 L_u^2 \E \|{z^t_i - \bar{u}^t }\|^2  
    +  3 \E \|{ \nabla_u F(\bar{u}^t,v^{t+1}) }\|^2  \\
    &+&  3\E \|{ \nabla_u F_i(\bar{u}^t,v^{t+1}) - \nabla_u F(\bar{u}^t,v^{t+1}) }\|^2 \notag\\
    &\overset{\text{Bounded Variance}}{\leq} & 3 L_u^2 \E \|{z^t_i - \bar{u}^t }\|^2  
     + 3 \E \|{ \nabla_u F(\bar{u}^t,v^{t+1}) }\|^2  + 3\delta_u^2
\end{eqnarray*}
\end{proof}

\begin{lemma}
\label{th:lemma4}
\begin{eqnarray}
M^{t}_i = \frac{1}{m}\sum^m_{i=1} \E \|{\bar{u}^t - z^t_i }\|^2 &\leq 
& \left( \eta_u^2 \frac{9 C^2}{(1 - q)^2} + \eta_u \frac{q^t 3 C^2}{1-q} \right) \delta_u^2  \notag\\
	& + & \left( \eta_u^2 \frac{9 L^2 C^2}{1 - q} + \eta_u q^t 3 L^2 C^2 \right) \sum^t_{j=0} q^{t-j} M^j_i  \notag\\
	& + &\left( \eta_u^2 \frac{9 C^2}{1 - q} + \eta_u q^t 3 C^2 \right) \sum^t_{j=0} q^{t-j} \E \|{ \nabla f(\bar{u}^j,v^{j+1}) }\|^2  \notag\\
	& + & \left(q^{2t} C^2 + \eta_u q^t \frac{2 C^2}{1-q} \right)  \frac{\sum^m_{i=1}\|  u_i^0 \|^2}{m}
\end{eqnarray}
\end{lemma}

\begin{proof}
    \begin{eqnarray}
    \E \|{\bar{u}^t - z^t_i }\|^2 &\overset{Lemma~\ref{th:lemma2}} {\leq}& \E \left( \underbrace{C q^t \|{ u_i^{0}}\|}_{a}  
    + \underbrace{ \eta_u C \sum^t_{s=0} q^{t-s} \|{ \nabla_u F_{i}(z_i^s,v^{s+1})\|} }_{b} \right)^2 \\
    %& \leq &  \E \left( C q^t \|{ u_i^0} \|  + \eta_u C \sum^t_{s=0} q^{t-s} \| \nabla F_{i}(z_i^s;\xi_i^s)- \nabla  F_i(z_i^s) + \nabla  F_i(z_i^s) )\| \right)^2 
    %&\leq& \E \left( \underbrace{C q^t \|x_i^0 \| }_{a}  + \underbrace{\eta_u C \sum^t_{s=0} q^{t-s} \|{\nabla  F_i(z^s_i,v^{s+1} \|}}_{b} + \underbrace{\eta_u C \sum^t_{s=0} q^{t-s} \|{ \ssgrad{i}{\vz}{\xi}{s} - \nabla f_i(\itr{\vz}{s})}}_{c} \| \right)^2  \notag\\
\end{eqnarray}

since $\E \|{\bar{u}^t - z^t_i }\|^2\leq \E(a^2 +b^2 + 2ab)$. Let us now obtain
bounds for the above inequality:

\begin{align*}
	a^2 &=  C^2 q^{2t} \|{ u_i^{0}}\|^2 \\
        b^2 &= \eta_u^2 C^2 \sum^t_{j=0} q^{2(t - j)} \|{ \nabla_u  F_i(z^j_i,v^{j+1}) }\|^2 +  \underbrace{2 \eta_u^2 C^2 \sum^t_{j=0} \sum^t_{s=j + 1} q^{2t -j - s} \| \nabla_u  F_i(z^j_i,v^{j+1})\| \| \nabla_u F_i(z^s_i,v^{s+1}) }_{b_1}\| \\
        2ab &= 2 \eta_u C^2 q^t \| u_i^0\| \sum^t_{s=0} q^{t-s} \| \nabla_u F_i(z^s_i,v^{s+1}) \| \\
\end{align*}

The expression $b_1$ is bounded as follows:
\begin{align}
\label{th:lemma4_b1}
    b_1 &= \eta_u^2 C^2 \sum^t_{j=0} \sum^t_{s=j + 1} q^{2t -j - s} 2 \|{ \nabla_u  F_i(z^j_i,v^{j+1}) }\| \|{ \nabla_u  F_i(z^s_i,v^{s+1}) }\| \notag\\
	&\overset{(ii)}{\leq} \eta_u^2 C^2 \sum^t_{j=0} \sum^t_{s=j+1} q^{2t - s - j}  \|{ \nabla_u  F_i(z^j_i,v^{j+1}) }\|^2 \notag_u \quad 
     + \eta_u^2 C^2 \sum^t_{j=0} \sum^t_{s=j+1} q^{2t - s - j} \|{ \nabla_u  F_i(z^s_i,v^{s+1}) }\|^2 \notag\\
	&\leq \eta_u^2 C^2 \sum^t_{j=0} q^{t - j} \|{ \nabla_u  F_i(z^j_i,v^{j+1}) }\|^2 \sum^t_{s=0} q^{t - s} \quad
     + \eta_u^2 C^2 \sum^t_{s=0} q^{t - s}  \|{ \nabla_u  F_i(z^s_i,v^{s+1}) }\|^2 \sum^t_{j=0} q^{t - j} \notag\\
	&\overset{(iii)}{\leq} \frac{1}{1 - q} \eta_u^2 C^2 \sum^t_{j=0} q^{t - j}  \|{ \nabla_u  F_i(z^j_i,v^{j+1}) }\|^2 \quad 
     +  \frac{1}{1-q} \eta_u^2 C^2 \sum^t_{s=0} q^{t -s} \|{ \nabla_u  F_i(z^s_i,v^{s+1}) }\|^2 \notag\\
	&=  \frac{2}{1 - q} \eta_u^2 C^2 \sum^t_{j=0} q^{t - j}  \|{ \nabla_u  F_i(z^j_i,v^{j+1}) }\|^2. 
\end{align}
where $(ii) \label{th:ii}$ and $(iii) \label{th:iii}$ is gotten from $\|x\|\|y\|\leq \frac{(\|x\|^2+\|y\|^2)}{2}$ and $\sum^K_{t=1}r^t \leq \sum^\infty_{t=1}r^t = \frac{1}{1-r}, r\in (0,1)$.

Thus,
\begin{eqnarray}
    b^2&=&\eta_u^2 C^2 \sum^t_{j=0} q^{2(t - j)} \|{ \nabla_u  f_i(z^j_i,v^{j+1}) }\|^2 + b_1 \notag\\
    & \leq &\frac{ \eta_u^ 2 C^2 }{1- q} \sum^t_{j=0} q^{t-j} \|{ \nabla_u  f_i(z^j_i,v^{j+1}) }\|^2 + b_1\notag\\
    &\overset{(\ref{th:lemma4_b1})}{\leq} & \frac{3 \eta_u^2 C^2}{1 - q} \sum^t_{j=0} q^{t-j} \|{ \nabla_u  f_i(z^j_i,v^{j+1}) }\|^2
\end{eqnarray}
Then let us bound the products $2ab$,
\begin{eqnarray}
	2ab &=& \eta_u C^2 q^t \sum^t_{s=0} q^{t-s} 2\|{ \nabla_u  f_i(z^j_i,v^{j+1}) }\| \notag\\
	&\overset{(ii)}{\leq}&\eta_u C^2 q^t \sum^t_{j=0} q^{t-j} \|{ \nabla_u  f_i(z^j_i,v^{j+1}) }\|^2 
        + \eta_u C^2 q^t \sum^t_{j=0} q^{t-j} \|u_i^0\|^2 \notag\\
	&\overset{(iii)}{\leq}& \eta_u C^2 q^t \sum^t_{j=0} q^{t-j} \|{ \nabla_u  f_i(z^j_i,v^{j+1}) }\|^2 
        + \frac{\eta_u C^2 \|u_i^0\|^2} {1 - q} q^{t}
\end{eqnarray}
By combining all of the above bounds together we obtain:
\begin{eqnarray}
	 \E \|{\bar{u}^t - z^t_i }\|^2 &\leq& \E(a^2 +b^2 + 2ab)\notag\\
        &\leq   & C^2 \|u_i^0\|^2 q^{2t} 
        +\frac{ \eta_u C^2 \|u_i^0\|^2}{1-q} q^t \notag\\
        & +&\E \frac{3 \eta_u^2 C^2}{1 - q} \sum^t_{j=0} q^{t-j}\|{ \nabla_u  f_i(z^j_i,v^{j+1}) }\|^2  
        + \E \eta_u C^2 q^t \sum^t_{j=0} q^{t-j}  \|{ \nabla_u  f_i(z^j_i,v^{j+1}) }\|^2 \notag\\
        &\leq & \left(q^{2t} C^2 
        + \eta_u q^t \frac{2 C^2}{1-q} \right)  \|u_i^0\|^2 
        + \left( \eta_u^2 \frac{3 C^2}{1 - q} 
        + \eta_u q^t C^2 \right) \sum^t_{j=0} q^{t-j} \E \|{ \nabla_u  f_i(z^j_i,v^{j+1}) }\|^2 \notag\\
        &\overset{Lemma~\ref{th:lemma3}}{\leq} &  \left(q^{2t} C^2 + \eta_u q^t \frac{2 C^2}{1-q} \right)  \|u_i^0\|^2 
        + \left( \eta_u^2 \frac{12 C^2}{(1 - q)^2} 
        + \frac{\eta_u q^t 3 C^2}{1 - q} \right) \delta^2 \notag\\
	& + &\left( \eta_u^2 \frac{9 L^2 C^2}{1 - q} + \eta_u q^t 3 L^2 C^2 \right) \sum^t_{j=0} q^{t-j} \E \|{\bar{u}^j - z^j_i }\|^2  \notag\\
	& + &\left( \eta_u^2 \frac{9 C^2}{1 - q} + \eta_u q^t 3 C^2 \right) \sum^t_{j=0} q^{t-j} \E \|{ \nabla_u  f_i(\bar{u}^j,v^{j+1}) }\|^2 
\end{eqnarray}
Thus,
\begin{eqnarray}
   M^{t}_i = \frac{1}{m}\sum^m_{i=1} \E \|{\bar{u}^t - z^t_i }\|^2 &\leq 
        & \left( \eta_u^2 \frac{9 C^2}{(1 - q)^2} + \eta_u \frac{q^t 3 C^2}{1-q} \right) \delta_u^2  \notag\\
	& + & \left( \eta_u^2 \frac{9 L^2 C^2}{1 - q} + \eta_u q^t 3 L^2 C^2 \right) \sum^t_{j=0} q^{t-j} M^j_i  \notag\\
	& + &\left( \eta_u^2 \frac{9 C^2}{1 - q} + \eta_u q^t 3 C^2 \right) \sum^t_{j=0} q^{t-j} \E \|{ \nabla_u f(\bar{u}^j,v^{j+1}) }\|^2  \notag\\
	& + & \left(q^{2t} C^2 + \eta_u q^t \frac{2 C^2}{1-q} \right)  \frac{\sum^m_{i=1}\|  x_i^0 \|^2}{m}
\end{eqnarray}
\end{proof}

\begin{lemma}
Let Assumptions 1-3 hold and let us define $D_2=1 - \dfrac{\eta_u^2 9 L^2 C^2}{(1-q)^2} - \dfrac{\eta_u 3 L^2 C^2}{(1-q)^2}$ . Then,
    \begin{eqnarray}
        \sum^{T}_{t=1} M^t &  \leq & \frac{ C^2}{(1-q)^2}  \frac{\sum^m_{i=1} \|x_i^0 \|^2}{m}  
    \end{eqnarray}
\end{lemma}

\begin{proof}
Using the bound for $Q^k_i$ let us first bound its average across all nodes $M^k$
\begin{eqnarray}
    M^{t}_i = \frac{1}{m}\sum^m_{i=1} \E \|{\bar{u}^t - z^t_i }\|^2 &\leq 
    & \left( \eta_u^2 \frac{9 C^2}{(1 - q)^2} + \eta_u \frac{q^t 3 C^2}{1-q} \right) \delta_u^2  \notag\\
    & + & \left( \eta_u^2 \frac{9 L^2 C^2}{1 - q} + \eta_u q^t 3 L^2 C^2 \right) \sum^t_{j=0} q^{t-j} M^j_i  \notag\\
    & + &\left( \eta_u^2 \frac{9 C^2}{1 - q} + \eta_u q^t 3 C^2 \right) \sum^t_{j=0} q^{t-j} \E \|{ \nabla_u f(\bar{u}^j,v^{j+1}) }\|^2  \notag\\
    & + & \left(q^{2t} C^2 + \eta_u q^t \frac{2 C^2}{1-q} \right)  \frac{\sum^m_{i=1}\|  u_i^0 \|^2}{m}
\end{eqnarray}

At this point note that for any $\lambda \in (0,1)$, non-negative integer $T \in \mathbb{N}$, and non-negative sequence ${\beta^j} \}_{j=0}^t$, it holds that
\begin{eqnarray}
\label{naosnao}
\sum^T_{t=1} \sum^t_{j=0} \lambda^{t-j} \beta^j  &=& \beta^0 \left( \lambda^T + \lambda^{T-1} + \cdots + \lambda^0 \right) +\beta^1 \left( \lambda^{T-1} + \lambda^{T
 - 2} + \cdots + \lambda^{0} \right) +\cdots+ \beta^T \left( \lambda^0 \right) \notag\\
&\leq & \frac{1}{1-\lambda} \sum^T_{j=0} \beta^j. 
\end{eqnarray}
Similarly,
\begin{eqnarray}
\label{ansjka}
\sum^T_{t=1} \lambda^t \sum^t_{j=0} \lambda^{t-j} \beta^j  = \sum^T_{t=1} \sum^t_{j=0} \lambda^{2t-j} \beta^j \leq \sum^T_{t=1} \sum^t_{j=0} \lambda^{2(t-j)} \beta^j &\overset{(\ref{naosnao})}{\leq}& \frac{1}{1-\lambda^2} \sum^T_{j=0} \beta^j
\end{eqnarray}

Now by summing from $t=1$ to $T$ and using the bounds of (\ref{naosnao}) and (\ref{ansjka}) we obtain:
\begin{align*}
	\sum^{T}_{t=1} M^t \leq&  \left( \eta_u^2 \frac{12 C^2}{(1 - q)^2} \right) \delta_u^2 T + \left( \frac{\eta_u 3 C^2}{1 - q} \right) \delta_u^2 \\
	& + \left( \frac{ C^2}{1-q^2} + \eta_u \frac{2C^2}{(1-q)^2} \right) \frac{\sum^m_{i=1} \|  u_i^0 \|^2}{m} \\
	& + \left( \eta_u^2 \frac{12 C^2}{(1 - q)^2} + \eta_u \frac{3 C^2}{1-q^2} \right) \sum^{T}_{t=1} \E \| \nabla f(\bar{u}^t,v^{t+1}) \|^2  \\
	& + \left( \eta_u^2 \frac{12 L^2 C^2}{(1 - q)^2} + \eta_u \frac{3 L^2 C^2}{1-q^2} \right) \sum^{T}_{t=1} M^t.
\end{align*}

By rearranging:
\begin{align*}
	\left( 1-\eta_u^2 \frac{9 L^2 C^2}{(1 - q)^2} - \eta_u \frac{3 L^2 C^2}{1-q^2} \right) \sum^{T}_{t=0} M^t \leq&  \left( \eta_u^2 \frac{12 C^2}{(1 - q)^2} \right) \delta_u^2 T + \left( \frac{\eta_u 3 C^2}{(1 - q)^2} \right) \delta_u^2 \\
	& + \left( \frac{ C^2}{1-q^2} + \eta_u \frac{2C^2}{(1-q)^2} \right) \frac{\sum^m_{i=1} {\| u_i^0\|} ^2}{m} \\
	& + \left( \eta_u^2 \frac{12 C^2}{(1 - q)^2} + \eta_u \frac{3 C^2}{1-q^2} \right) \sum^{T}_{t=0} \E \|{ \nabla f(\bar{u}^t,v^{t+1}) \| }^2  \\
\end{align*}

Note that since $q\in (0,1)$, it holds that $\frac{1}{1-q^2}\leq \frac{1}{(1-q)^2}$.\footnote{This step is used to simplify the expressions involved the parameter $q$. One can still obtain similar results by keeping the expression $\frac{1}{1-q^2}$ in the definition of $D_2$.}  Thus, assume $\eta_u \ll \frac{1-q^2}{3C^2}$ and $D_2 = \left( 1-\eta_u^2 \frac{9 L^2 C^2}{(1 - q)^2} - \eta_u \frac{3 L^2 C^2}{1-q^2} \right) \approx 1$ we have,
\begin{align*}
	\sum^{T}_{t=1} M^t &\leq\left( \eta_u^2 \frac{9 C^2}{(1 - q)^2D_2} \right) \delta_u^2 T 
        + \left(\eta_u  \frac{ 3 C^2}{(1 - q)^2 D_2} \right) \delta_u^2 \\
        & + \left( \frac{ C^2}{(1-q)^2D_2} 
        + \eta_u \frac{2C^2}{(1-q)^2D_2} \right) \frac{\sum^m_{i=1} \|u_i^0 \|^2}{m} \\
        & + \left( \eta_u^2 \frac{12 C^2}{(1 - q)^2 D_2} 
        + \eta_u \frac{3 C^2}{(1-q)^2 D_2} \right) \sum^{T}_{t=1} \E \| \nabla_u f(\bar{u}^t,v^{j+1}) \|^2 \\
        & \leq  \frac{ C^2}{(1-q)^2}  \frac{\sum^m_{i=1} \|x_i^0 \|^2}{m}  
\end{align*}
The proof is completed.
\end{proof}

\subsection{Proof of Convergence Analysis}
\textbf{Proof Outline and the Challenge of Dependent Random Variables.}
    We start with 
    \begin{align} 
        \begin{aligned}
        F\left(\Bar{u}^{t+1}, V^{t+1}\right)
        - F\left(\Bar{u}^{t}, V^{t}\right)
        =&\, F\left(\Bar{u}^{t}, V^{t+1}\right)
        - F\left(\Bar{u}^{t}, V^{t}\right) \\
        &+ F\left(\Bar{u}^{t+1}, V^{t+1}\right)
        - F\left(\Bar{u}^{t}, V^{t+1}\right) \,.
        \end{aligned}
    \end{align}
    The first line corresponds to the effect of the $v$-step and the second line to the $u$-step. The former is 
    \begin{equation}
        \begin{split}
            F\left(\Bar{u}^{t}, V^{t+1}\right)
        - F\left(\Bar{u}^{t}, V^{t}\right) & = \frac{1}{m}\sum_{i=1}^m \E \Big[F_i(\Bar{u}^t, v_i^{t+1} ) - F_i(\Bar{u}^t, v_i^{t} )\Big]\\
        & \le 
        \frac{1}{m}\sum_{i=1}^m \E \Big[
        \Big <\nabla_v F_i\left(\Bar{u}
        ^{t}, v^{t}_i\right), v^{t+1}_i - v^{t}_i \Big>
        + \frac{L_v}{2}\|v^{t+1}_i - v^{t}_i \|^2 \Big] \,.
        \end{split}
    \end{equation}
    It is easy to handle with standard techniques that rely on the smoothness of $F\left(u^{t}, \cdot\right)$. 
    The latter is more challenging. 
    In particular, the smoothness bound for the $u$-step gives us
    \begin{align}
        F&\left(\Bar{u}^{t+1}, V^{t+1}\right)
        - F\left(\Bar{u}^{t}, V^{t+1}\right)
        \le 
        \Big <\nabla_u F\left(\Bar{u}
        ^{t}, V^{t+1}\right), \Bar{u}^{t+1} - \Bar{u}^{t} \Big>
        + \frac{L_u}{2}\|\Bar{u}^{t+1} - \Bar{u}^{t}\|^2 \,.
    \end{align}
    
\subsubsection{Proof of Convergence Analysis for DFedAlt}

\textbf{Analysis of the $u$-Step.}
    \begin{align} 
        \begin{aligned}
        & \E \Big [F\left(\Bar{u}^{t+1}, V^{t+1}\right)
        - F\left(\Bar{u}^{t}, V^{t+1}\right) \Big]
         \le 
        \Big <\nabla_u F\left(\Bar{u}
        ^{t}, V^{t+1}\right), \Bar{u}^{t+1} - \Bar{u}^{t} \Big>
        + \frac{L_u}{2}\E\|\Bar{u}^{t+1} - \Bar{u}^{t}\|^2\\
        & \leq \frac{-\eta_u}{m}\sum_{i=1}^m\E\Big <\nabla_u F\left(\Bar{u}
        ^{t}, V^{t+1}\right), \sum_{k=0}^{K_u-1}\nabla_u F\left(z_i^{t,k}, v_i^{t+1}; \xi_i\right)\Big> 
        + \frac{L_u}{2}\E\|\Bar{u}^{t+1} - \Bar{u}^{t}\|^2\\
        & \leq -\eta_uK_u \E [\Delta_{\Bar{u}}^t] + \frac{\eta_u}{m}\sum_{i=1}^m\sum_{k=0}^{K_u-1} \E \Big< \nabla_u F\left(\Bar{u}^{t}, V^{t+1}\right), \nabla F\left(\Bar{u}^t, v_i^{t+1}\right) - \nabla_u F\left(z_i^{t,k}, v_i^{t+1}; \xi_i\right) \Big> + \frac{L_u}{2}\E\|\Bar{u}^{t+1} - \Bar{u}^{t}\|^2 \\
        & \overset{ii)}{\leq} \frac{-\eta_uK_u }{2} \E [\Delta_{\Bar{u}}^t] + \underbrace{\frac{\eta_uL_u^2}{2m}\sum_{i=1}^m\sum_{k=0}^{K_u-1} \E \| z_i^{t,k} - \Bar{u}^t \|^2}_{\mathcal{T}_{1, u}} + \underbrace{\frac{L_u}{2}\E\|\Bar{u}^{t+1} - \Bar{u}^{t}\|^2}_{\mathcal{T}_{2, u}}.
        \end{aligned}
    \end{align}

 Where a) uses $\E\left[ \nabla_u F(u_i^{t,k}, v_i^{t+1}; \xi_i) \right]= \nabla_u F\left(u_i^{t,k}, v_i^{t+1}\right)$ and $\left<x, y\right> \leq \frac{1}{2}\|x\|^2 + \frac{1}{2}\|y\|^2 $ for vectors $x, y$ followed by $L_u$-smoothness.\\
 
For $\mathcal{T}_{1, u}$, we can use Lemma\ref{th:lemma4}:
\begin{equation}\label{T1_u}
    \begin{split}
        \mathcal{T}_{1, u} \leq \mathcal{T}_{1, u} &= \frac{\eta_uL_u^2 K_u}{2} M^t
    \end{split}
\end{equation}

Meanwhile, for $\mathcal{T}_{2, u}$,
    \begin{align} 
        \begin{aligned}
         \mathcal{T}_{2, u} & \leq \frac{\eta_u^2L_u}{2m} \sum_{i=1}^m\sum_{k=0}^{K_u-1}\Big \|\nabla_u F\left(z_i^{t,k}, v_i^{t+1}; \xi_i\right) - 
         \nabla_u F\left(z_i^{t}, v_i^{t+1}\right) + \nabla_u F\left(z_i^{t}, v_i^{t+1}\right) \\
        & - \nabla_u F\left(\bar{u}_i^{t}, V^{t+1}\right) + \nabla_u F\left(\bar{u}_i^{t}, V^{t+1}\right) - \nabla_u F\left(\Bar{u}^{t} , V^{t+1}\right) + \nabla_u F\left(\Bar{u}^{t}, V^{t+1}\right)\Big \|^2 \\
        &  \leq 2\eta_u^2K_uL_u\Big(  \sigma_z^2+\delta_v^2+\frac{L_u^2}{m}\sum_{i=1}^m\sum_{k=0}^{K_u-1}\E \|z_i^{t}-\Bar{u}^{t}\|^2 + \E[\Delta_{\Bar{u}}^t] \Big)\\
        &  \leq 2\eta_u^2K_uL_u\Big(  \sigma_z^2+\delta_v^2+ \E[\Delta_{\Bar{u}}^t] \Big)+2\eta_u^2K_uL_u^3  M^t
        \end{aligned}
    \end{align}

%%%%%%%%%%%%%%%%%%%%%%%%%%%%%%%%%%%%%%%%%%%%%%%%%%%%%%%%%%%%%%%%%%%%%%%%
Thus,
\begin{equation}
    \begin{split}
        \E \Big [F\left(\Bar{u}^{t+1}, V^{t+1}\right)
        - F\left(\Bar{u}^{t}, V^{t+1}\right) \Big]
         & \le \frac{-\eta_uK_u}{2}\E[\delta_v{\Bar{u}}^t] + \mathcal{T}_{1, u} + \mathcal{T}_{2, u}\\
         & \le \Big( \frac{-\eta_uK_u}{2} + 2\eta_u^2K_uL_u \Big)\E[\delta_v{\Bar{u}}^t] \\
         &+ 2\eta_u^2K_uL_u(\sigma_u^2+\delta_v^2) \\
         &  + \Big(2\eta_u^2K_uL_u^3+ \frac{\eta_uL_u^2 K_u}{2}  \Big)M^t.
    \end{split}
\end{equation}

\textbf{Analysis of the $v$-Step.}
\begin{equation}
        \begin{split}
           \E \Big [ F\left(\Bar{u}^{t}, V^{t+1}\right)
        - F\left(\Bar{u}^{t}, V^{t}\right) \Big]
        &  \le  \underbrace{\frac{1}{m}\sum_{i=1}^m \E 
        \Big <\nabla_v F_i\left(\Bar{u}
        ^{t}, v^{t}_i\right), v^{t+1}_i - v^{t}_i \Big>}_{\mathcal{T}_{1, v}}
        + \underbrace{\frac{L_v}{2m}\sum_{i=1}^m \E  \|v^{t+1}_i - v^{t}_i \|^2 }_{\mathcal{T}_{2, v}}.
        \end{split}
    \end{equation}
For $\mathcal{T}_{1, v}$, 
\begin{equation}\label{eq:T_1_a}
    \begin{split}
       \mathcal{T}_{1, v} & \leq \frac{1}{m}\sum_{i=1}^m \E 
        \Big <\nabla_v F_i\left(\Bar{u}
        ^{t}, v^{t}_i\right) - \nabla_v F_i\left(z_i
        ^{t}, v^{t}_i\right) + \nabla_v F_i\left(z_i
        ^{t}, v^{t}_i\right), -\eta_v \sum_{k=0}^{K_v-1} \E \nabla_v F_i(u_i^t, v^{t}_i; \xi_i) \Big> \\
        & \overset{a)}{\leq} \frac{-\eta_vK_v}{m}\sum_{i=1}^m \E \| \nabla_v F_i(u_i^t, v^{t}_i) \|^2 + \frac{1}{m}\sum_{i=1}^m \E 
        \Big <\nabla_v F_i\left(\Bar{u}
        ^{t}, v^{t}_i\right) - \nabla_v F_i\left(z_i
        ^{t}, v^{t}_i\right), v^{t+1}_i - v^{t}_i \Big> \\
        & \overset{b)}{\leq} -\eta_vK_v \E [\Delta_v^t] + \underbrace{\frac{L_{vu}^2}{2m}\sum_{i=1}^m \E \|\Bar{u}^t-z_i^{t}\|^2}_{\mathcal{T}_{3, v}} + \underbrace{\frac{1}{2m}\sum_{i=1}^m \E \|v^{t+1}_i - v^{t}_i\|^2}_{\frac{1}{L_v}\mathcal{T}_{2, v}},
    \end{split}
\end{equation}
where a) and b) is get from the unbiased expectation property of $\nabla_v F_i(u_i^{t},v^{t}_i; \xi_i)$  and $<x, y> \leq \frac{1}{2}(\|x\|^2+\|y\|^2)$, respectively.

For $\mathcal{T}_{2, v}$, according to Lemma \ref{le:v}, we have 
\begin{equation}\label{eq:T_2_a}
    \begin{split}
       \mathcal{T}_{2, v} & \leq \frac{L_v}{2}\Big( \frac{16 \eta_v^2 K_v^2}{m}\sum_{i=1}^m \E \|\nabla_v F_i(u_i^t, v^{t}_i)\|^2 + 8 \eta_v^2 K_v^2 \sigma_v^2\Big)\\
       & \leq   8L_v\eta_v^2 K_v^2 \E [\Delta_v^t] + 4L_v\eta_v^2 K_v^2 \sigma_v^2.
    \end{split}
\end{equation}

For $\mathcal{T}_{3, v}$, according to Lemma \ref{th:lemma4}, we have 
\begin{equation}\label{eq:T_3_a}
    \frac{L_{vu}^2}{2m}\sum_{i=1}^m \E \|\Bar{u}^t-z_i^{t}\|^2 \leq  \frac{L_{uv}^2}{2} M^t.
\end{equation}

After that, summing Eq. (\ref{eq:T_1_a}), (\ref{eq:T_2_a}), and (\ref{eq:T_3_a}), we have
\begin{equation}
    \begin{split}
      \E \Big [ F\left(\Bar{u}^{t}, V^{t+1}\right)
        - F\left(\Bar{u}^{t}, V^{t}\right) \Big]  
        \le \Big(-\eta_vK_v + 8\eta_v^2K_v^2(L_v)\Big)\E [\Delta_v^t] +  4\eta_v^2K_v^2\sigma_v^2L_v + \frac{L_{uv}^2}{2} M^t.
    \end{split}
\end{equation}
% Using Eq. (\ref{T_1_u}), we have
\textbf{Obtaining the Final Convergence Bound.} 
\begin{align} \label{eq:pfl-am:pf:2}
        \begin{aligned}
       \E \Big [   F\left(\Bar{u}^{t+1}, V^{t+1}\right)
        - F\left(\Bar{u}^{t}, V^{t}\right)  \Big]  
        =&\,\E \Big [  F\left(\Bar{u}^{t}, V^{t+1}\right)
        - F\left(\Bar{u}^{t}, V^{t}\right) + F\left(\Bar{u}^{t+1}, V^{t+1}\right)
        - F\left(\Bar{u}^{t}, V^{t+1}\right)  \Big]    \\
        & \leq \Big( \frac{-\eta_uK_u}{2} + 2\eta_u^2K_uL_u\Big)\E[\Delta_{\Bar{u}}^t] \\
        &+ \Big(-\eta_vK_v + 8\eta_v^2K_v^2 L_v\Big)\E [\Delta_v^t] \\
         &  + 2\eta_u^2K_uL_u(\sigma_u^2+\delta_v^2)  +  4\eta_v^2K_v^2\sigma_v^2L_v \\
        & +   \Big(2\eta_u^2K_uL_u^3+ \frac{\eta_uL_u^2 K_u + L^2_{uv}}{2}  \Big)M^t.
        \end{aligned}
    \end{align}
Summing from $t=1$ to $T$, assume the local learning rates satisfy $\eta_u=\mathcal{O}({1}/{L_uK_u\sqrt{T}}), \eta_v=\mathcal{O}({1}/{L_vK_v\sqrt{T}})$, $F^{*}$ is denoted as the minimal value of $F$, i.e., $F(\bar{u}, V)\ge F^*$ for all $\bar{u} \in \mathbb{R}^{d}$, and $V=(v_1,\ldots,v_m)\in\mathbb{R}^{d_1+\ldots+d_m}$. We can generate
\begin{equation}
    \begin{split}
        \frac{1}{T}\sum_{i=1}^T \bigl(\frac{1}{L_u} \E \bigl[\Delta_{\bar{u}}^t \bigr] + \frac{1}{L_v} \E [\Delta_{v}^t \bigr] \bigr) 
        & \leq \mathcal{O}\Big(\frac{F(\bar{u}^1, V^1) - F^*}{\sqrt{T}} 
        + \frac{\sigma_v^2}{L_v\sqrt{T}}
        + \frac{\sigma_u^2+\delta_v^2}{L_u K_u\sqrt{T}}  \\
        & + \frac{(L_u+L^2_{uv}) C^2 \sum^m_{i=1}\|u_i^0\|^2 }{ m (1-q^2) \sqrt{T}} 
        +  \frac{L_u C^2 \sum^m_{i=1}\|u_i^0\|^2 }{ K_u m (1-q^2) \sqrt{T^3}} \Big).
    \end{split}
\end{equation}
Assume that
\begin{align}
        \sigma_1^2 = \frac{\sigma_v^2}{L_v} 
        +  \frac{\sigma_u^2+\delta_v^2}{L_u K_u}
        +\frac{(L_u+L^2_{uv}) C^2 \sum^m_{i=1}\|u_i^0\|^2 }{ m (1-q^2)}, ~~~
         \sigma_2^2 = \frac{L_u C^2 \sum^m_{i=1}\|u_i^0\|^2 }{ K_u m (1-q^2) }
\end{align}
Then, we have the final convergence bound:
\begin{equation} 
\small
    \frac{1}{T}\sum_{i=1}^T \bigl(\frac{1}{L_u} \E \bigl[\Delta_{\bar{u}}^t \bigr] 
    + \frac{1}{L_v} \E [\Delta_{v}^t \bigr] \bigr) \leq \mathcal{O}\Big(\frac{F(\bar{u}^1, V^1) - F^*}{\sqrt{T}} 
    + \frac{\sigma_1^2}{\sqrt{T}} 
    + \frac{\sigma_2^2}{\sqrt{T^3}} \Big).
\end{equation}
